# Supplementary material for: NMR-based gap behavior related to the quantum size effect
Source: arXiv:2003.07585 source file (2020-03-17)
Supplement: Supplementary file 1 [file Supplemental.pdf]

## Supplementary Information

# NNR-based gap behavior related to the quantum size effect

Tomonori Okuno, Masahiro Manago, Shunsaku Kitagawa, and Kenji Ishida  
Kohei Kusada, and Hiroshi Kitagawa

### I. Sample condition

The Pt nanoparticles coated with polyvinylpyrrolidone (PVP) were prepared by the reduction of metal ions with alcohol under aqueous conditions without the requirement for any harmful organic reagent. This was done by dissolving 3.0 mmol of  $\text{K}_2\text{PtCl}_4$  in deionized water. Then, PVP and a reducing agent (ethylene glycol (EG) or triethylene glycol (TEG)) were added to the  $\text{K}_2\text{PtCl}_4$  solution. The solution was then heated to a certain temperature and held at that temperature for 1.5 h. The color of the precursor solution then slowly changed to black, indicating the formation of Pt nanoparticles. After the completion of the reaction, the prepared nanoparticles were separated by centrifuging. Size control was achieved by adjusting the concentrations of the reagents and the PVP, as well as the temperature used for the synthesis (TAB. S1)

Transmission electron microscopy (TEM) images of the PVP-coated nanoparticles are shown in Fig. S1 (a). Using these TEM images, the average and variance of the diameter of the four nanoparticle samples were determined. The results are shown in Fig. S1 (b) as a histogram. For all four samples, the distribution of the diameter is around 15 %. To investigate the crystal structure, X-ray diffraction XRD measurements were carried out at room temperature. The results are shown in Fig. S2.

TABLE S1 Reaction Conditions for Synthesis of Pt Nanoparticles

|               | <b>H<sub>2</sub>O</b><br><b>(ml)</b> | <b>Reducing agent</b><br><b>(ml)</b> | <b>PVP</b><br><b>(mmol)</b> | <b>Temperature</b><br><b>(°C)</b> |
|---------------|--------------------------------------|--------------------------------------|-----------------------------|-----------------------------------|
| <b>2.5 nm</b> | 40                                   | EG / 100                             | 9                           | 120                               |
| <b>4.0 nm</b> | 40                                   | TEG / 125                            | 9                           | 120                               |
| <b>7.4 nm</b> | 3                                    | TEG / 75                             | 9                           | 200                               |
| <b>9.8 nm</b> | 1.5                                  | TEG / 75                             | 15                          | 200                               |

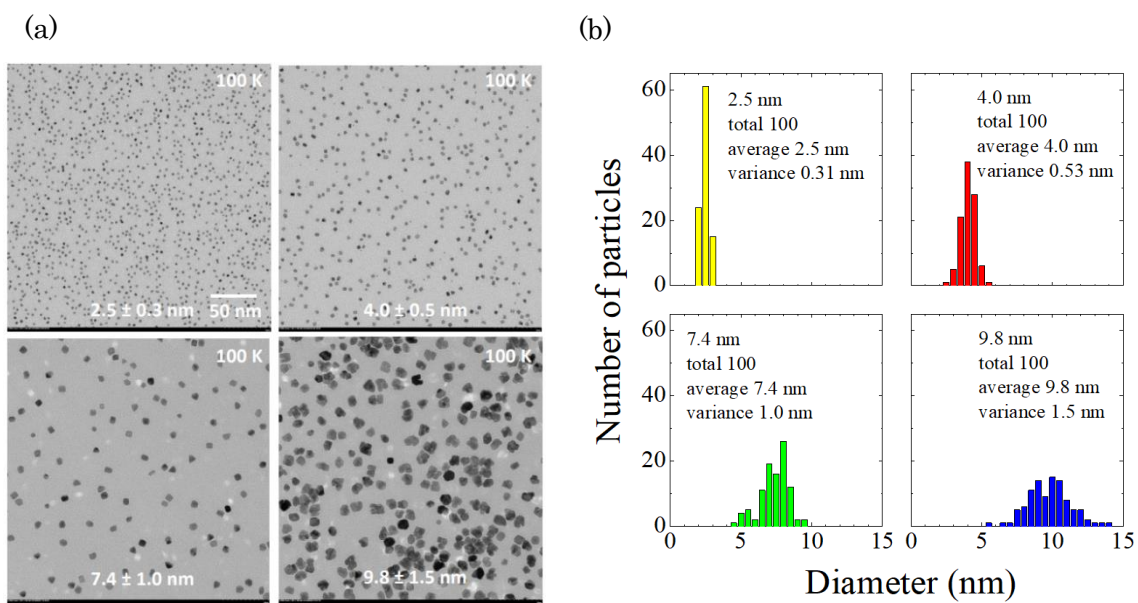

FIG. S1. (a) TEM images of PVP-coated Pt nanoparticles. (b) Histograms of nanoparticle size for each sample.

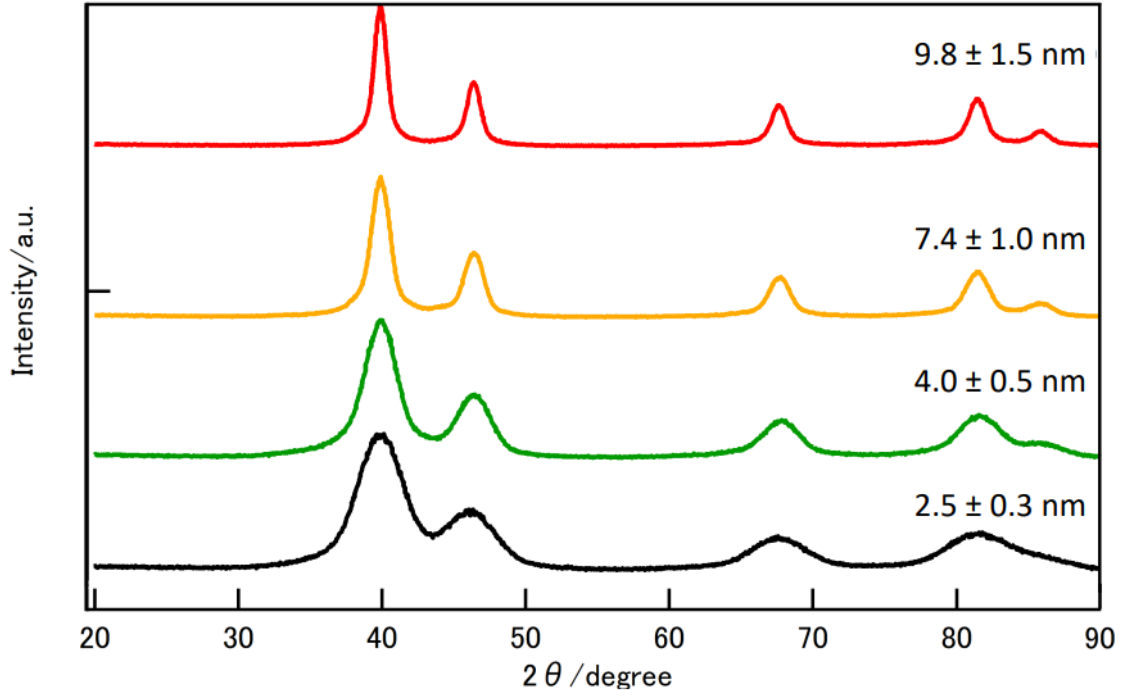

FIG. S2. XRD patterns of four Pt nanoparticles.

## II. Recovery curves of nuclear magnetization for evaluation of nuclear spin-lattice relaxation time $T_1$

The nuclear spin-lattice relaxation time  $T_1$  is the time constant which describes the exchange of nuclear spin energy with the surrounding electronic system.  $T_1$  is measured with the recovery of the nuclear spin after the saturation of the nuclear spin. Because the nuclear spin of  $^{195}\text{Pt}$  is  $I = 1/2$ , the recovery curve  $R(t) \equiv [M(\infty) - M(t)]/M(\infty)$  of the nuclear magnetization  $M(t)$  is fitted to a single exponential function

$$\frac{M(\infty) - M(t)}{M(\infty)} = \exp\left(-\frac{t}{T_1}\right),$$

in the metallic temperature region, as shown in FIGs. S3 (a) and (b).

For the recovery curve at low temperatures ( $< 4$  K),  $R(t)$  cannot be fitted to the single exponential function. To enable a quantitative discussion, the fastest and slowest components were fitted as shown in FIG. S3 (c).

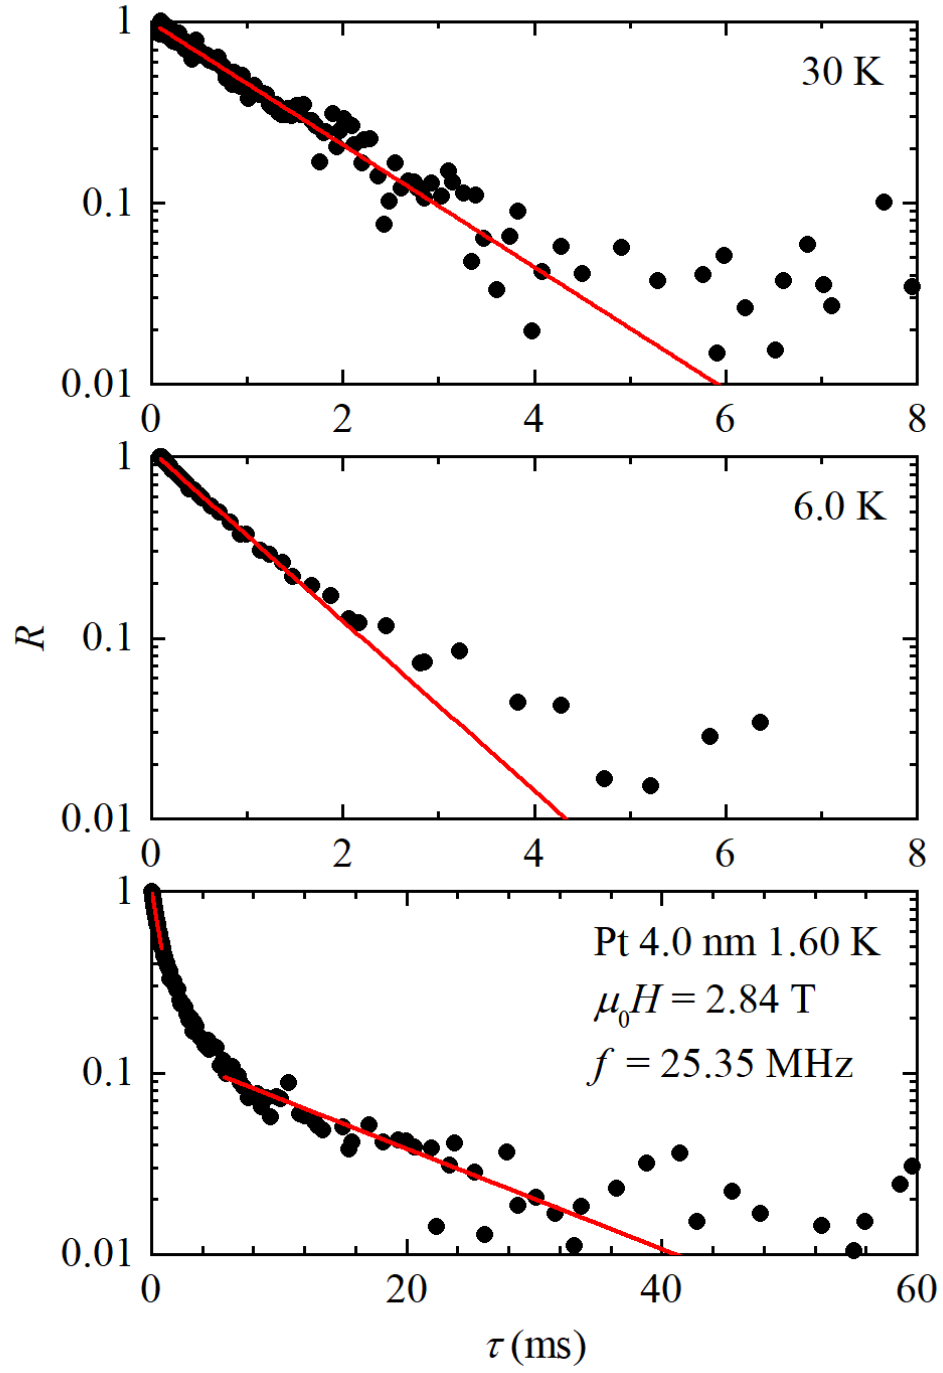

FIG. S3. Recovery curves  $R(t)$  of the 4.0-nm-diameter Pt nanoparticle sample at various temperatures: 30 K (metallic region), 6.0 K ( $< T^*$ ), and 1.60 K (below the peak temperature). The solid lines are fitted by a single exponential function

### III. Heating effects

For the spin-echo method, we applied two RF pulses. Generally, the RF pulses heat the sample. The heating effects sometimes lead to multi-recovery. With the goal of eliminating this possibility, in this section we discuss the heating effects. This concern is frequently discussed in the case of bulk metal materials, in which the eddy current induced by the RF-pulses causes Joule heating.

In the case of nanoparticles, the heating effect is less likely. In general, because the heating effect is usually caused by the eddy current, this effect is small in powdered samples, especially insulating samples. As nanoparticles are “ultimately” powdered samples, heating is less likely. In addition, as our data suggested (and which would be theoretically expected), nanoparticles would be insulating at low temperatures, such that a heating effect would not be expected.

Experimentally, we have checked whether the results are changed by varying the energy of the RF-pulses. Figure S4 shows the NMR spectra of 4.0-nm samples at a temperature of 1.55 K. As the energy of the RF-pulses decreases, even to the point where the intensity of the NMR signal becomes so small that the signal-to-noise ratio worsens, the shape of the spectrum does not change. Figures S5 and S6 show the recovery curves of the nuclear magnetization obtained by using RF pulses of various energies at temperatures of 8.0 and 1.60 K, respectively. When we decreased the energy of the RF pulses, the recovery curves did not change at all. Therefore, in the considered range of energies, the heating effects were negligibly small.

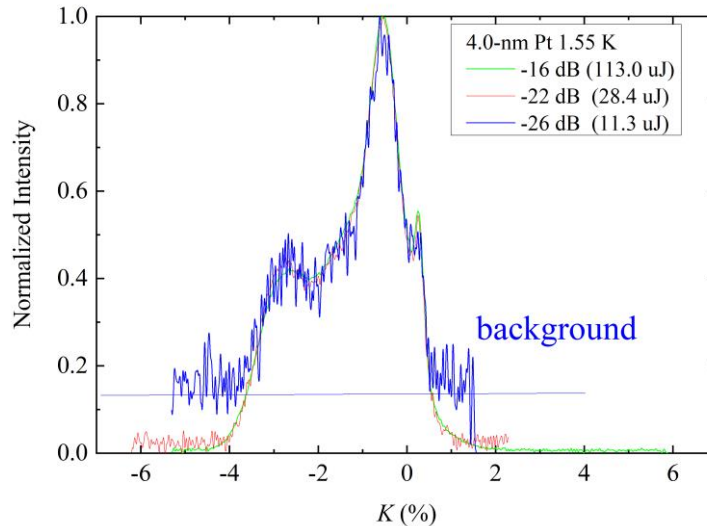

FIG. S4: Normalized NMR spectrum of 4.0-nm samples obtained using RF pulses of different powers

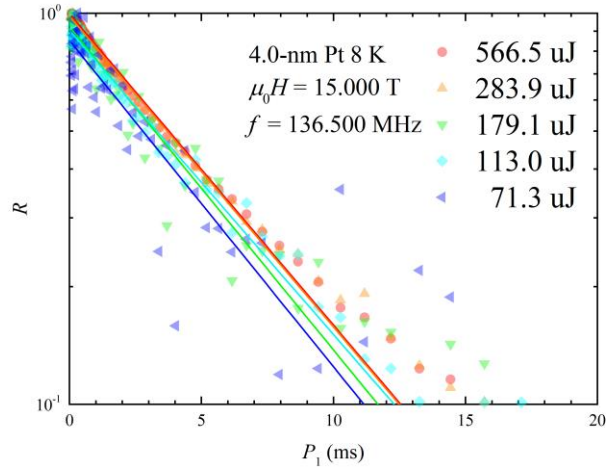

FIG. S5: Recovery curves of 4.0-nm samples at 8.0 K, obtained using RF pulses of different powers. Solid lines: fitting lines.

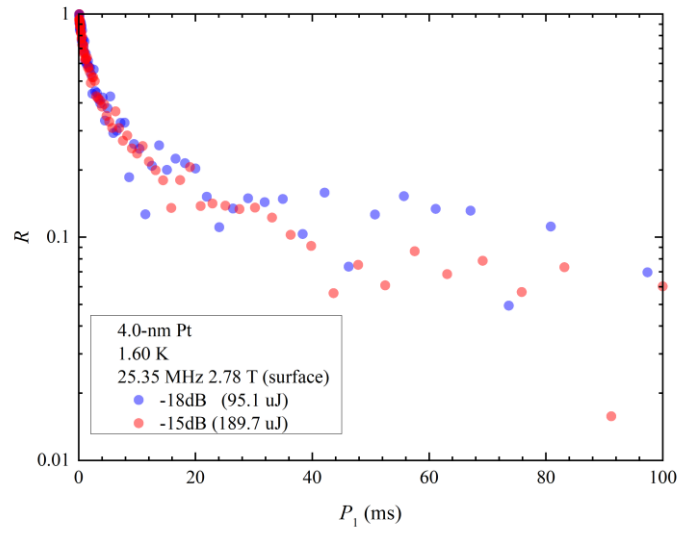

**Fig. R5:** Recovery curves of 4.0-nm samples at 1.60 K, obtained using RF pulses of different powers.
